# Supplementary material for: Near threshold all-optical backaction amplifier
Source: arXiv:1109.2004 source file (2011-09-09)
Supplement: Supplementary file 1 [file SuppplementRMA.tex]

\documentclass[12pt]{iopart}
\usepackage{graphicx,amssymb,amsfonts}

%Uncomment next line if AMS fonts required
%\usepackage{iopams}
\begin{document}

%\title{Ch6 Optomechanical regenerative amplification}

%,amsmath,amssymb,amsfonts

\title{Supplementary information}
\section{Coupled equations of motion}
When the optical cavity resonance frequency is blue detuned from the laser frequency, that is ($\Delta_0=\Omega-\Omega_0>0$) where $\Omega_0$ is the cavity resonance  in the absence of mechanical coupling and $\Omega$ is the optical pump frequency,  the radiation pressure force shifts the cavity further off resonance reducing the intracavity power and consequently the radiation pressure. The lower radiation pressure now allows the cavity to spring back toward resonance leading to periodic oscillations when the input optical power is above a threshold level. The radiation pressure force is given by $F_{rp}=g\hbar |a|^2$ where the stored cavity phonon number is denoted by $|a|^2$ and the optomechanical coupling strength is given by $g=\Omega_0/\rm{r}$ where $r$ is the radius of the toroid.  This radiation pressure mediated interaction between the optical and mechanical degrees of freedom in a cavity optomechanical system can result in regenerative amplification. This process can be described by the following two coupled equations of motion \cite{KippenbergOptExp} when the sidebands are within the optical linewidth, as is the case for these results,

%\begin{equation}\label{eq:MechanicalLangevin} %eq (1) notes
%\dot{a}=-\left[\gamma-i \left(\Delta_{0}+\frac{\Omega_{0} x}{R}+\Lambda |a|^{2} \right)\right]a+\sqrt{2\gamma_{\rm{in}}}a_{\rm{in}}+\sqrt{2\gamma_{\rm{l}}}a_{\rm{l}}
%\label{MechanicalLangevin}
%\end{equation}

\begin{equation}\label{eq:MechanicalLangevin} %eq (1) notes
\dot{a}=-\left[\gamma-i \left(\Delta_{0}+gx  +\Lambda |a|^{2} \right)\right]a+\sqrt{2\gamma_{\rm{in}}}a_{\rm{in}}+\sqrt{2\gamma_{\rm{loss}}}a_{\rm{loss}}
\label{MechanicalLangevin}
\end{equation}

\begin{equation}\label{eq:DDO} %eq (2) notes
\ddot{x}+\Gamma \dot{x} + \Omega_{m}^2 x = g\frac{\hbar}{m_{\rm{eff}}}|a|^2+\frac{F_T}{m_{\rm{eff}}}
\label{DDO}
\end{equation}

The coordinate around which the mechanical oscillations are centered is given by the nominal cavity length $x$ and the optical decay rate of the cavity, $\gamma$, is equal to the sum of the input coupling rate, $\gamma_{\rm{in}}$, and the cavity loss rate, $\gamma_{\rm{loss}}$, that is $\gamma=\gamma_{\rm{in}}+\gamma_{\rm{loss}}$. The intrinsic mechanical damping coefficient is given by $\Gamma$, $\Omega_m$ is the mechanical resonance frequency of the mechanical mode driven by the optical field and $m_{\rm{eff}}$ is the associated effective vibrating mass of the mechanical mode. The optical field Kerr effect is parameterized by the rate $\Lambda$. $F_T$ is the Langevin force to account for the Brownian motion and satisfies the fluctuation dissipation theorem and can be explained conveniently in the frequency domain as $F_T(\Omega)=\sqrt{2m_{\rm{eff}}\Gamma k_B T}\xi(\Omega)$ where $k_B$ is Boltzmann's constant, $T$ is the temperature and $\xi$ is a unit of white noise. The zero point mechanical motion is $x_{\rm{zp}}=\sqrt{\frac{\hbar}{2m_{\rm{eff}}\Omega_m}}$ and the phonon occupation number is given in the high temperature limit of relevance here by $\bar{n}=\frac{k_B T}{\hbar\Omega_m}$. It is convenient to define the following dimensionless parameters for analysis: $\tilde{\Omega}=\Omega/\gamma$, $\tilde{\Delta}=\bar{\Delta}/\gamma$, $\tilde{r}=r/x_{zp}$, $\tilde{a}_{in}=a_{in}/\sqrt{2\gamma}$, $\tilde{\xi}(\Omega)=\tilde{\xi}(\Omega)/\sqrt{\gamma}$, $\eta=\gamma_{in}/\gamma$, $\gamma=\gamma_{\rm{in}}+\gamma_{\rm{loss}}$ $\tilde{x}=x/x_{zp}$, and $\tilde{g}=gx_{\rm{zp}}/\gamma$.

\section{Linearization}
As the optical or mechanical fluctuations are small relative to their steady state amplitudes we can solve eqs.(\ref{MechanicalLangevin}) and (\ref{DDO}) by linearization. We will write optical field amplitude as $a(t)=\bar{a}+\delta a(t)$, where $\bar{a}$ is a complex number representing the classical steady state (mean field) component and $\delta a(t)$ represents the time varying fluctuations. Similarly the mechanical displacement $x(t)=\bar{x}+\delta x(t)$ is also linearized. Linearisation then involves neglecting the small higher order terms, such that for example we approximate $|a|^2 = |\bar{a}|^2 + \delta a^{\dagger}\bar{a} + \delta \bar{a}a^{\dagger}$. We can similarly linearize the mechanical field and show in the next section the mean cavity length change $\bar{x}$ is coupled to a mean frequency shift $\bar{\Delta}$.

\subsection{Optical mean field in the steady state}
We first consider the mean optical field where the steady state has been reached the steady state of the radiation pressure, that is $\langle\dot{a}\rangle=\dot{\bar{a}}=0$ and $\langle\dot{a}\rangle=\dot{\bar{a}}=0$, where the bar is used throughout to denote the mean field. Using Eqn.(\ref{MechanicalLangevin}) it is then straight forward to show that this leads to the mean field amplitude in the resonator 
\begin{equation}\label{eq:MeanPhononNumber}%eq (8) notes
\bar{a}=\frac{\sqrt{2\gamma_{\rm{in}}}\bar{a}_{\rm{in}}}{\gamma-i\bar{\Delta}}
\label{MeanPhononNumber}
\end{equation}
where the mean field detuning is defined as
\begin{equation}\label{eq:MeanPDetuning}%eq (8) notes
\bar{\Delta} \equiv \Delta_0+\frac{\Omega_0 \bar{x}}{R}+\Lambda|\bar{a}|^2.
\label{MeanDetuning}
\end{equation}
The input-output relation \cite{WallsMilburn1994} $(a_{\rm{out}}=\sqrt{2\gamma_{\rm{in}}}a-a_{\rm{in}})$ then leads to
\begin{equation}\label{eq:DimensionlessMeanPhononNumber}%eq (12) notes
\tilde{\bar{a}}_{\rm{out}}=\tilde{\bar{a}}_{\rm{in}}\left[\frac{2\eta}{1-i\tilde{\Delta}}-1\right],
\label{DimensionlessMeanPhononNumber}
\end{equation}
where we have switched to dimensionless units denoted by the tildes.

\subsection{Optical field fluctuations}
Equation (\ref{MechanicalLangevin}) is linearized then transformed into the frequency domain with the Fourier transform properties $F(\dot{g}(t))=i\omega F(g(t))$ and $F(a^*(t))=a^*(-\Omega)$. We introduce the additional dimensionless parameters $\tilde{\Lambda}=\Lambda/\gamma$, $K=\tilde{\Lambda|\bar{a}|^2}$, $M=\tilde{\Omega_0}|\bar{a}|/\tilde{r}$ and rearrange the expression in terms of the optical field fluctuations.
\begin{eqnarray}\label{eq:MechanicalLangevinNoise}%eq (28) notes
\delta a(\Omega)&=&\tilde{\chi}_{opt}[M\sqrt{L}(J(\Omega)+i)\delta x(\Omega)+2\sqrt{\eta}\delta\tilde{a}_{\rm{in}}(\Omega)\\ \nonumber
&+&2iJ(\Omega)L\sqrt{\eta}\delta\tilde{a}^{\dagger}_{\rm{in}}(-\Omega)+2\sqrt{1-\eta}\delta\tilde{a}_{\rm{loss}}(\Omega)\\ \nonumber
&+&2iJ(\Omega)L\sqrt{1-\eta}\delta\tilde{a}^{\dagger}_{\rm{loss}}(-\Omega) ]\\ \nonumber
\label{MechanicalLangevinNoise}
\end{eqnarray}
where it is convenient to define the following terms
\begin{equation}\label{eq:J}%eq (27) notes
J\equiv\frac{K}{1+i(\tilde{\Omega}+\tilde{\Delta}^*+K^*)},
%\label{J}
\end{equation}
\begin{equation}\label{eq:L}%eq (27) notes
L=(1+i\tilde{\Delta})/(1-i\tilde{\Delta})
\label{L}
\end{equation}
and the optical susceptibility
\begin{equation}\label{eq:K}
\tilde{\chi}_{opt}\equiv[1+i(\tilde{\Omega}-\tilde{\Delta}-K)-K^*J]^{-1}.
\label{K}
\end{equation}

\subsection{Mechanical field fluctuations}
A similar linearisation and Fourier transform of Eq.(\ref{DDO}) yields the frequency domain mechanical fluctuations
%where the motion of the mirror is assumed to be simple harmonic
%We now consider the mechanical fluctuations in the cavity at the SQL, where $x_{\rm{zp}}$ and the linearization of equation \ref{DDO} give \textbf{the fourier component of the resonant displacement}
%\begin{equation}\label{eq:DimensionlessSusceptibility}
%\delta\tilde{x}(\Omega)x_{\rm{zp}} = \frac{\tilde{\chi}(\Omega)}{m\gamma^2}\left[ \left( \frac{\hbar\tilde{\Omega_{0}}\gamma}{\tilde{R}x_{\rm{zp}}} \right) (\bar{a}\delta{a}^{\dagger}(-\Omega) + %\bar{a}^*\delta a(\Omega)) + \sqrt{2m \Gamma k_B T \gamma} \hat{\xi} (\Omega)\right].
%\label{ZeroPointFluctuations}
%\end{equation}
\begin{equation}\label{eq:DisplacementNoise1}%eq (42) notes
\delta\tilde{x}(\Omega)=2\tilde{\Omega}_m\tilde{\chi}(\Omega)[M(\sqrt{L}\delta a^{\dagger}(-\Omega)+\sqrt{L^*}\delta a(\Omega)+\sqrt{\bar{n}\tilde{\Gamma}}\tilde{\xi}(\Omega))].
\label{DisplacementNoise1}
\end{equation}
Where the mechanical susceptibility is a measure of the mechanical deformation to an applied force. From Eq.(\ref{DDO}) we introduce a dimensionless mechanical susceptibility $\tilde{\chi}(\Omega)=M\gamma^2\chi(\Omega)$ where
\begin{equation}\label{eq:DimensionlessSusceptibility}
\tilde{\chi}(\Omega)=\frac{\gamma^2}{\Omega_m^2-\Omega^2+i\Omega\Gamma}.
\label{DimensionlessSusceptibility}
\end{equation}
As the optical field fluctuations are a function of the mechanical fluctuations we substitute Eq.(6) and it's adjoint into Eq.(\ref{DisplacementNoise1}) to give
\begin{eqnarray}\label{eq:DisplacementNoise2}%eq (36) and (41)
\fl\delta\tilde{x}(\Omega)&\!=\!2\tilde{\Omega}_m\tilde{\chi}_{\rm{eff}}(\Omega)[2\sqrt{L^*}M(\tilde{\chi}_{\rm{opt}}(\Omega)\!-\!iJ^*(\!-\Omega)\chi^*_{\rm{opt}}(\!-\Omega))[\sqrt{\eta}\delta \tilde{a}_{\rm{in}}(\Omega)\!+\!\!\sqrt{1\!\! -\! \eta}\delta \tilde{a}_{\rm{l}}(\Omega)] \\ \nonumber
\fl&+\!2\sqrt{L}M(\tilde{\chi}^*_{\rm{opt}}(-\Omega)\!+\!i J(\Omega)\chi_{\rm{opt}}(\Omega))[\sqrt{\eta}\delta a^*_{\rm{in}}(-\Omega)\!+\!\sqrt{1\!-\!\eta}\delta a^*_{\rm{l}}(-\Omega)]\!+\!\sqrt{\bar{n}\bar{\Gamma}}\tilde{\xi}(\Omega)]
\label{DisplacementNoise2}
\end{eqnarray}
%I think I will stop the full solution around here and continue with J=K=0 ie no Kerr effect as the full solution is done numerically on the computer anyway.
where the mechanical susceptibility is modified by the presence of the optical field to%eq (42)
\begin{equation}\label{eq:DimensionlessEffectiveSusceptibility}%eq (42) notes
\fl\tilde{\chi}^{-1}_{eff}(\Omega)\equiv\tilde{\chi}^{-1}(\Omega)-2\tilde{\Omega}_m M^2[\tilde{\chi}^*_{opt}(-\Omega)(J^*(-\Omega)-i))+\tilde{\chi}_{opt}(\Omega)(J(\Omega)+i)]
\label{DimensionlessEffectiveSusceptibility}
\end{equation}
which can be written in the general Lorentzian form

\begin{equation}\label{eq:DimensionlessEffectiveSusceptibility}%eq (42) notes
\tilde{\chi}_{\rm{eff}} = \frac{G_1}{\Omega^{\prime 2}_{\rm{m}} - \Omega^2 + i G_2 \Omega \Gamma (1-R)}.
\label{DimensionlessEffectiveSusceptibility2}
\end{equation}
With the effect of the optical field to modify the mechanical resonance frequency $\Omega^{\prime}_{m}$, scale the Lorentzian by a constant factor $G_1$, and introduce an amplification factor $R$ which offsets the intrinsic loss of the oscillator, where $R=1$ is the regenerative amplification threshold.

%A factor $G_2$ modifies the mechanical damping of the oscillator which is reduced as the power, $P$, is increased towards the regenerative amplification threshold ($R=1$).}

\section{Output field quadratures for optomechanical system}
To eventually take account of the sensitivity of the system to a measurement of the change in the cavity length a signal is now included which perturbs the cavity length by a small amount $x_{\rm{sig}}$, consequently the optomechanical coupling term, $gx$, in Eq.(\ref{MechanicalLangevin}) is modified to $g(x+x_{\rm{sig}})$. By substituting Eq.(\ref{DisplacementNoise2}) into Eq.(6) and using the input output relation we arrive at an expression for the dimensionless field output as measured by the photodetector.
%\textbf{This outgoing field includes both the mirror and signal displacement noise.}
%(ie eq (52) notes)

%probably skip the next 19 lines
%Here however, we will continue with the assumption of no optical Kerr effect, i.e. K=J=0, this assumption will lead to relatively simple expressions for the output field quadratures. With no Kerr %effect the effective susceptibility is now
%\begin{equation}\label{eq:EffectiveSusceptibilityK0} %eq (63) notes
%\chi_{eff}=\frac{G}{\tilde{\Omega}_m^{\prime2}-\Omega^2+i\tilde{\Omega}\tilde{\Gamma}^{\prime}}
%\label{EffectiveSusceptibilityK0}
%\end{equation}
%where
%\begin{equation}\label{eq:G} %eq (64) notes
%G=\left [1+\frac{4\tilde{\Omega}_mm^2\tilde{\Delta}}{|\Upsilon|^2}\right ]^{-1}
%\label{G}
%\end{equation}
%\begin{equation}\label{eq:DimensionlessEffectiveMechanicalFrequency} %eq (64) notes
%\tilde{\Omega}^{\prime2}_m=\tilde{\Omega}^2_m\left[1+\frac{4m^2\tilde{\Delta}(1+\tilde{\Delta}^2)}{|\Upsilon|^2\tilde{\Omega}_m}G\right]
%\label{DimensionlessEffectiveMechanicalFrequency}
%\end{equation}
%\begin{equation}\label{eq:DimensionlessEffectiveMechanicalDamping} %eq (64) notes
%\tilde{\Gamma}^{\prime2}_m=\tilde{\Gamma}\left[1-\frac{8\tilde{\Omega}_m m^2\tilde{\Delta}}{|\Upsilon|^2\tilde{\Gamma}}G\right]
%\label{DimensionlessEffectiveMechanicalDamping}
%\end{equation}

\begin{eqnarray}\label{eq:DimensionlessFieldOut}%eq (52)
\fl\delta\tilde{a}_{\rm{out}}=C_1 \delta\tilde{a}_{\rm{in}}(\Omega)+C_2\delta\tilde{a}^{\dagger}_{\rm{in}}(-\Omega)+C_3\xi(\Omega)+C_4\delta\tilde{a}_{\rm{loss}}(\Omega)+C_5\delta\tilde{a}^{\dagger}_{\rm{loss}}(-\Omega)+C_6\delta x_{\rm{sig}}
\label{DimensionlessFieldOut}
\end{eqnarray}
where
\begin{eqnarray}\label{eq:C}%eq (52) expanded in terms of variables "b"
\fl C_1=\eta(2\tilde{\chi}_{\rm{opt}}[1+2\tilde{\Omega}_{\rm{m}}\tilde{\chi}_{\rm{eff}}M^2(J(\Omega)+1)(\tilde{\chi}_{\rm{opt}}-iJ^*(-\Omega)\tilde{\chi}^*_{\rm{opt}}(-\Omega))])-1\\ \nonumber
\fl C_2=\eta(2\tilde{\chi}_{\rm{opt}}L[i J(\Omega)+2\tilde{\Omega}_{\rm{m}}\tilde{\chi}_{\rm{eff}}M^2(J(\Omega)+1)(\tilde{\chi}^*_{\rm{opt}}(-\Omega)+i J(\Omega)\tilde{\chi}_{\rm{opt}}(\Omega))])\\ \nonumber
\fl C_3=\sqrt{\eta}(2\tilde{\Omega}_{\rm{m}}\tilde{\chi}_{\rm{eff}}M \sqrt{L}(J(\Omega)+1)\sqrt{\tilde{n}\tilde{\Gamma}}\tilde{\chi}_{\rm{opt}}(\Omega))\\ \nonumber
\fl C_4=\sqrt{\eta(1-\eta)}(2\tilde{\chi}_{\rm{opt}}[1+2\tilde{\Omega}_{\rm{m}}\tilde{\chi}_{\rm{eff}}M^2(J(\Omega)+1)(\tilde{\chi}_{\rm{opt}}-iJ^*(-\Omega)\tilde{\chi}^*_{\rm{opt}}(-\Omega))])\\ \nonumber
\fl C_5=\sqrt{\eta(1-\eta)}(2\tilde{\chi}_{\rm{opt}}L[i J(\Omega)+2\tilde{\Omega}_{\rm{m}}\tilde{\chi}_{\rm{eff}}M^2(J(\Omega)+1)(\tilde{\chi}^*_{\rm{opt}}(-\Omega)+i J(\Omega)\tilde{\chi}_{\rm{opt}}(\Omega))])\\ \nonumber
\fl C_6=\frac{iM}{2}\sqrt{\eta}[\sqrt{L}(2\tilde{\chi}_{\rm{opt}}[1+2\tilde{\Omega}_{\rm{m}}\tilde{\chi}_{\rm{eff}}m^2(J(\Omega)+1)(\tilde{\chi}_{\rm{opt}}-iJ^*(-\Omega)\tilde{\chi}^*_{\rm{opt}}(-\Omega))]) \\ \nonumber
-\sqrt{L^*}(2\tilde{\chi}_{\rm{opt}}L[i J(-\Omega)+2\tilde{-\Omega}_{\rm{m}}\tilde{\chi}_{\rm{eff}}M^2(J(-\Omega)+1)(\tilde{\chi}^*_{\rm{opt}}(\Omega)+i J(-\Omega)\tilde{\chi}_{\rm{opt}}(-\Omega))])                                                                                        ]\\ \nonumber
\label{C}
\end{eqnarray}
From \cite{WallsMilburn1994} we use the following expression to calculate the output field amplitude quadrature
\begin{equation}\label{eq:GeneralQuadrature}%eq (80) notes
X^{+}_{\rm{out}}(\Omega)=e^{i\phi}a^*_{\rm{out}}(-\Omega)+e^{-i\phi}a_{\rm{out}}(\Omega)
\label{GeneralQuadrature}
\end{equation}
where we are doing a self homodyne measurement so $\phi$ is the delay on the mean field due to the cavity.
From Eq.(\ref{DimensionlessMeanPhononNumber}) we find that $e^{i\phi}=\frac{2\eta}{1-i\tilde{\Delta}}-1=L_2$ and rewrite the output field quadrature as
\begin{equation}\label{eq:GeneralQuadrature}%eq (83) notes
X^{+}_{\rm{out}}(\Omega)=L_2a^*_{\rm{out}}(-\Omega)+L^*_2a_{\rm{out}}(\Omega)
\label{GeneralQuadrature}
\end{equation}
We now substitute the output field fluctuations measured by the detector, Eq.(\ref{DimensionlessFieldOut}), into the above expression and  rearrange to get
\begin{equation}\label{eq:GeneralQuadratureH}%eq (86) notes
\fl X^{+}_{\rm{out}}(\Omega)=H_1\delta a_{\rm{in}}(\Omega)+H_2\delta a^{\dagger}_{\rm{in}}(-\Omega)+H_3\xi(\Omega)+H_4\delta a_{\rm{l}}(\Omega)+
H_5\delta a^{\dagger}_{\rm{l}}(-\Omega)+\sqrt{2\gamma}H_6\delta\tilde{x}_{\rm{sig}}
\label{GeneralQuadratureH}
\end{equation}
where
\begin{eqnarray}\label{eq:H}
H_1=L_2C^*_2(-\Omega)+L_2^*C_1(\Omega)\\ \nonumber
H_2=L_2C^*_1(-\Omega)+L_2^*C_2(\Omega)\\ \nonumber
H_3=L_2C^*_3(-\Omega)+L_2^*C_3(\Omega)\\ \nonumber
H_4=L_2C^*_5(-\Omega)+L_2^*C_4(\Omega)\\ \nonumber
H_5=L_2C^*_4(-\Omega)+L_2^*C_5(\Omega)\\ \nonumber
H_6=L_2C^*_6(-\Omega)+L_2^*C_6(\Omega).\\ \nonumber
\label{H}
\end{eqnarray}
Using the quadrature expressions \cite{WallsMilburn1994}%ie (87)(88) are already given in intro so this package ties together nicely
\begin{equation}\label{eq:GeneralQuadratureH}%eq (86) notes
\delta a_{\rm{in}}(\Omega)=\frac{X^+_{\rm{in}}(\Omega) + i X^-_{\rm{in}}(\Omega)}{2}
\label{GeneralQuadratureHplus}
\end{equation}
\begin{equation}\label{eq:GeneralQuadratureH}%eq (86) notes
\delta a^{\dagger}_{\rm{in}}(-\Omega)=\frac{X^+_{\rm{in}}(\Omega) + i X^-_{\rm{in}}(\Omega)}{2},
\label{GeneralQuadratureHminus}
\end{equation}
Eq.(\ref{GeneralQuadratureH}) can be rearranged into the form
\begin{eqnarray}\label{eq:GeneralQuadratureH2a}%eq (90) notes
X^+_{\rm{out}}(\Omega)&=X^+_{\rm{in}}(\Omega)\frac{H_1+H_2}{2}+iX^-_{\rm{in}}(\Omega)\frac{H_1-H_2}{2}+X^+_{\rm{loss}}(\Omega)\frac{H_4+H_5}{2} \\ \nonumber
&+iX^-_{\rm{loss}}(\Omega)\frac{H_4-H_5}{2}+H_3\xi(\Omega)+\frac{\sqrt{2\gamma}}{x_{\rm{zp}}}H_6\delta\tilde{x}_{\rm{sig}}\\ \nonumber
&=X^+_{\rm{in}}(\Omega)G^+_{\rm{in}} + iX^-_{\rm{in}}(\Omega)G^-_{\rm{in}} + X^+_{\rm{loss}}(\Omega)G^+_{\rm{loss}} \\ \nonumber
&+X^-_{\rm{loss}}(\Omega)G^-_{\rm{loss}} + H_3\xi(\Omega) + \frac{\sqrt{2 \gamma}}{x_{\rm{zp}}} H_6 \delta \tilde{x}_{\rm{sig}}.
\label{GeneralQuadratureH2a}
\end{eqnarray}
%where $G^{\pm}_{\rm{in}}=\frac{H_1 \pm H_2}{2}$, $G^{\pm}_{\rm{loss}}=\frac{H_4 \pm H_5}{2}$
where
\begin{equation}\label{eq:GeneralQuadratureIn}%eq (86) notes
G^{\pm}_{\rm{in}}=\frac{H_1 \pm H_2}{2}
\label{GeneralQuadratureIn}
\end{equation}
and
\begin{equation}\label{eq:GeneralQuadratureIn}%eq (86) notes
G^{\pm}_{\rm{loss}}=\frac{H_4 \pm H_5}{2}.
\label{GeneralQuadratureIn}
\end{equation}
The amplitude $\hat{X}^+(\Omega)$ and the phase $\hat{X}^-(\Omega)$ quadratures obey the boson commutation relation $[\hat{X}^+(\Omega),\hat{X}^-(\Omega)] = 2i$ and $\Delta \hat{X}^{+}(\Omega) = \Delta \hat{X}^{-}(\Omega) = 1$ for the coherent states.

It can be immediately seen from Eq.(23) that the intensity transfer function, recorded on the network analyzer, is 
\begin{equation}\label{eq:AmplitudeTF}%eq (91) notes
\rm{T}_{\rm{intensity}}= \left| \frac{H_1+H_2}{2} \right| ^2
\label{AmplitudeTF}
\end{equation}
%and the phase transfer function is
%\begin{equation}\label{eq:PhaseTF}%eq (92) notes
%G^-=i\frac{H_1-H_2}{2}
%\label{PhaseTF}
%\end{equation}
%The output variance is a measure of the noise on the amplifier output and is a summation of the input amplitude and phase noise, the input loss amplitude and phase noise the mechanical oscillator and signal noise respectively and has the following form
%\begin{eqnarray}\label{eq:OutputVariance}%eq (93) notes
%V^{+}_{\rm{out}}(\Omega)&=V^+_{\rm{in}}(\Omega)\left| \frac{H_1+H_2}{2}\right|^2+V^-_{\rm{in}}(\Omega)\left|\frac{H_1-H_2}{2}\right|^2\\ \nonumber
%&+V^+_{\rm{loss}}(\Omega)\left|\frac{H_4+H_5}{2}\right|^2+V^-_{\rm{loss}}(\Omega)\left|\frac{H_4-H_5}{2}\right|^2\\ \nonumber
%&+\left|H_3\right|^2+\frac{2\gamma}{x^2_{\rm{zp}}}|H_6|^2V(\delta x_{\rm{sig}}).
%\label{OutputVariance}
%\end{eqnarray}

\section{Sensitivity beyond the standard quantum limit}
Following the method of Arcizet \emph{et. al.} \cite{ArcizetPinardBeatingSQL2006} we show that the measurement sensitivity to a change in cavity length can go beyond the standard quantum limit using the backaction of the optomechanical amplifier to modify the mechanical susceptibility.

%\begin{equation}\label{eq:GeneralQuadratureG}
%\delta a_{\rm{in}}(\Omega)=\frac{X^+_{\rm{in}}(\Omega) + iX^-_{\rm{in}}(\Omega)}{2}
%\label{GeneralQuadratureG}
%\end{equation}

%\begin{equation}\label{eq:GeneralQuadratureG}
%\delta a^+_{\rm{in}}(-\Omega)=\frac{X^+_{\rm{in}}(\Omega) - iX^-_{\rm{in}}(\Omega)}{2}
%\label{GeneralQuadratureG}
%\end{equation}

%\begin{equation}\label{eq:GeneralQuadratureG}
%\fl X^{+}_{\rm{out}}(\Omega)=X^+_{\rm{in}}(\Omega)G^+ + X^-_{\rm{in}}(\Omega)G^- + X^+_{\rm{loss}}(\Omega)G^+_{\rm{loss}} +  X^-_{\rm{loss}}(\Omega)G^-_{\rm{loss}} + \frac{\sqrt{2 %\gamma}}{x_{\rm{zp}}}H_6 \delta x_{\rm{sig}}.
%\label{GeneralQuadratureG}
%\end{equation}
Assuming the mirror is cooled such that thermal motion is negligible as in \cite{ArcizetPinardBeatingSQL2006} and rearranging Eq(23) for $\delta x_{\rm{sig}}$ we find
\begin{equation}\label{eq:SignalNoise}
\fl \delta x_{\rm{sig}}=\frac{x_{\rm{zp}}}{\sqrt{2 \gamma} H_6}\left[X^{+}_{\rm{out}}(\Omega)- X^+_{\rm{in}}(\Omega)G^+ - X^-_{\rm{in}}(\Omega)G^- - X^+_{\rm{loss}}(\Omega)G^+_{\rm{loss}} -  X^-_{\rm{loss}}(\Omega)G^-_{\rm{loss}}\right].
\label{SignalNoise}
\end{equation}
We can therefore make an estimate of the signal based on our measurement $X^+_{\rm{out}}(\Omega)$
\begin{equation}\label{eq:SignalNoiseEst}
\delta x_{\rm{sig,est}}=\frac{x_{\rm{zp}}}{\sqrt{2 \gamma} H_6} X^{+}_{\rm{out}}(\Omega)
\label{SignalNoiseEst}
\end{equation}
and the uncertainty in the measurement is
%$\langle  \delta X^+ \delta X^- \rangle = 0$
\begin{equation}\label{eq:SignalAmp}
S_{\rm{x,sig}}=\left\langle\left(\delta x_{\rm{sig}} - \delta x_{\rm{sig,est}}\right)^2\right\rangle
\label{SignalAmp}
\end{equation}
which for a coherent input state gives
\begin{equation}\label{eq:SignalAmp}
S_{\rm{x,sig}}=\frac{x^2_{\rm{zp}}}{\sqrt{2 \gamma} |H_6|^2}\left[ |G^+|^2 + |G^-|^2 + |G_{\rm{loss}}^+|^2 + |G_{\rm{loss}}^-|^2 \right].
\label{SignalAmp}
\end{equation}
Comparing this with the SQL, $S_{\rm{SQL}}=\hbar |\chi_{\rm{eff}}(\Omega)|$, \cite{ArcizetPinardBeatingSQL2006} we find

%\begin{equation}\label{eq:SignalAmpSQL}
%\frac{S_{\rm{x,sig}}}{S_{\rm{SQL}}}=\frac{x^2_{\rm{zp}}}{2 \gamma \hbar |\chi_{\rm{eff}}(\Omega)|}\left[ \frac{ |G^+|^2 + |G^-|^2 + |G_{\rm{loss}}^+|^2 + |G_{\rm{loss}}^-|^2 }{|H_6|^2}\right]
%\label{SignalAmpSQL}
%\end{equation}

%where $x^2_{\rm{zp}}=\frac{\hbar}{2\rm{m}\Omega_{\rm{m}}}$ and $\chi_{\rm{eff}}=\frac{\tilde{\chi}_{\rm{eff}}}{m \gamma^2}$ to give the result

\begin{equation}\label{eq:FinalSignalAmpSQL}
\frac{S_{\rm{x,sig}}}{S_{\rm{SQL}}}=\frac{1}{4\tilde{\Omega}_{\rm{m}}|\tilde{\chi}_{\rm{eff}}(\Omega)|}    \left[ \frac{ |G^+|^2 + |G^-|^2 + |G_{\rm{loss}}^+|^2 + |G_{\rm{loss}}^-|^2 }{|H_6|^2}\right].
\label{FinalSignalAmpSQL}
\end{equation}

%and the \textbf{cavity length modulation} caused by the signal we wish to measure is $x_{\rm{sig}}$.

\section{References}

\end{document}
